# Supplementary material for: Functional connectomes of neural networks
Source: arXiv:2412.15279 ancillary file (2025-04-11)
Supplement: Supplementary file 1 [file technical_appendix.pdf]

# Technical Appendix: Functional Connectomes of Neural Networks

## Baseline Methods

We explored six baseline methods. Four of these methods employ the k-medoids algorithm with the following distances and kernels: bottleneck distance (BD), Wasserstein distance (WD), sliced Wasserstein kernel (SWK) (Carriere, Cuturi, and Oudot 2017), and heat kernel (HK) (Reininghaus et al. 2015). These methods use the weighted adjacency matrices, also referred to as functional connectomes $C$, as input. From these, we compute persistence diagrams of cycles ($H_1$) using the `ripser` (Tralie, Saul, and Bar-On 2018) package. Since `ripser` expects distance matrices $D$ as input, the functional connectomes are converted to distance matrices via the formula $D = \sqrt{1 - C}$ (Songdechakraiwut and Chung 2023). This transformation captures the inverse relationship between correlation and distance while preserving the symmetry and triangle inequality of the distance matrix. We then calculate pairwise distance from persistence diagrams using the `persim` (Saul and Tralie 2021) package and perform k-medoids clustering. The default settings are used in both `ripser` and `persim`. The k-medroids algorithm is implemented in `sklearn_extra` (scikit-learn extra 2020) with the settings of `metric="precomputed"`, `init="random"`, `method="pam"`.

The other two use a k-means clustering algorithm on persistence image (PI) (Adams et al. 2017) vectorization and on the vectorization of entries below the main diagonal of the adjacency (Adj), respectively. Persistence Images are obtained from persistence diagrams using `PersistenceImager` in `persim` with settings `birth_range=(0, 1)`, `pers_range=(0, 1)`, `pixel_size=0.05`, which convert persistence diagrams to persistence images of $20 \times 20$ resolution. These images are then flattened into vectors. Euclidean distances between these vectors are computed to perform k-means clustering. K-means in `sklearn` (Pedregosa et al. 2011) is implemented with the settings of `init="random"`, `n_init=1`. `traditional_clustering_pipeline.py` provides more details on the implementation of BD, WD, SWK, HK, PI, and `clustering_pipeline.py` provides more detail on the implementation of Adj.

## Dataset

In order to investigate the functional behavior of neural networks, we performed our analyses on the MNIST (LeCun et al. 1998), Fashion-MNIST (Xiao, Rasul, and Vollgraf 2017), and CIFAR-10 (Krizhevsky, Hinton et al. 2009) datasets. These datasets are widely used in the context of image classification tasks. The datasets are directly obtained from `torchvision` (TorchVision 2016). The detailed implementation of dataset loading is available in the code as a part of the `loading_pipeline.py` script.

The MNIST dataset comprises grayscale images of handwritten digits from 0 to 9. Each image has a centered digit with a resolution of $28 \times 28$. The training set contains 60,000 examples, and the test set contains 10,000 examples. The Fashion-MNIST dataset consists of grayscale images of fashion items. The images are categorized into ten classes: T-shirt/top, trousers, pullover, dress, coat, sandal, shirt, sneaker, bag, and ankle boot. The dataset shares the same number of training and testing examples and the same image resolution as MNIST. The CIFAR-10 dataset consists of color images of ten classes of common objects and animals, including airplane, automobile, bird, cat, deer, dog, frog, horse, ship, and truck. Each image has three color channels with a resolution of $32 \times 32$. The training set contains 50,000 images, and the test set contains 10,000 images.

In our studies, each dataset is split into training and functional datasets. The training dataset is used to train networks, and the functional dataset is used to produce functional connectomes. We used one-sixth of the original training data as the functional dataset. The implementations slightly differ in the two studies. In the first study, a random split is implemented using `randperm` in `torch` (Paszke et al. 2019). In the second study, we implemented `StratifiedShuffleSplit` in `sklearn` in order to maintain the same distribution of classes in training and functional datasets. Both studies had a fixed seed for reproducibility. More details on the design of the two studies are described in Section 3 of the main text.

## Hyperparameter Tuning

Hyperparameter tuning selects the combination of hyperparameters that yields the most optimal performance for a model. It ensures the model is learning effectively. In our studies, we perform hyperparameter tuning using $k$-fold

cross-validation. The training dataset is divided into five equal parts, where four parts are used for training, and one part is used for testing. By comparing the test accuracies of all hyperparameter combinations, the optimal set of hyperparameter combinations is determined. The detailed implementation of $k$-fold cross-validation is available in the code as a part of the `training_pipeline.py` script.

The tuning process focused on four key hyperparameters, including the training epoch number ($e$), the negative slope coefficient ($\alpha$) in the leaky ReLU activation function (Maas et al. 2013), the regularization strength ($\lambda$) in $L^2$ regularization (Hoerl and Kennard 1970), and the dropout rate ($d$) (Srivastava et al. 2014). Specifically, $e$ represents the number of training iterations, $\alpha$ represents the negative slope coefficient applied to the negative input in Leaky ReLU, $\lambda$ represents the regularization rate that penalizes large weights $w_i$ in Loss $= \text{Error}(y, \hat{y}) + \lambda \sum_{i=1}^{N} w_i^2$ for $L^2$ regularization, and $d$ represents the probability of dropping out each neuron. The hyperparameters are given choices as follows.

| Hyperparameter | Choices |
|---|---|
| $e$ (training epoch) | 20, 30, 40 |
| $\alpha$ (LReLU slope) | 0.01, 0.1 |
| $\lambda$ ($L^2$ penalty) | 0.0001, 0.001, 0.005, 0.01 |
| $d$ (dropout rate) | 0.1, 0.2, 0.3, 0.4 |

Table 1: Hyperparameters Grid Search Choices

We adopted a grid search approach to search for the optimal model over predefined hyperparameters. First, the Cartesian product of different hyperparameters is calculated to define the grid search space. Then, models with sets of hyperparameter values are evaluated and compared based on the test accuracies. In the case where hyperparameters are shared across experiments, identical choices are offered in the grid search space. Since we are interested in the influence of regularization strategies in comparison to vanilla, these strategies are implemented separately in experiments where no two strategies are applied together. More details on hyperparameters and grid search can be found in `training_pipeline.py` and scripts of individual experiments.

There was a slight variation in how the training dataset was partitioned between the two studies. In the first study, we performed cluster analysis on regularization types with stimuli from all predefined classes. Thus, $k$-fold with $k = 5$ in `torch` was implemented to partition training data into folds completely randomly. In the second study, we performed cluster analysis on stimuli from specific classes. A stratified version of $k$-fold in `sklearn` was implemented so that it was randomly partitioned within each predefined class. This approach ensured that each fold maintained the same distribution of predefined classes.

## Additional Results of Study 1

In Study 1, we examined the influence of different regularization strategies on functional mechanisms, including batch normalization (Ioffe and Szegedy 2015), dropout, and $L^2$. For each strategy and the control group *vanilla*, we trained 20 neural networks. Then, we inputted the functional dataset into each trained network and extracted a functional connectome from it. This process resulted in 20 connectomes per regularization strategy. We then conducted cluster analysis on these functional connectomes with varying topological weights $\lambda$ (Songdechakraiwut et al. 2022). $\lambda$ represents the degree to which topological information influences the interpolation between Adj and Top. When $\lambda = 0$, the algorithm only utilizes geometric information, representing the method Adj. When $\lambda = 1$, the method only uses topological information, corresponding to the method Top.

The clustering performance was assessed using purity scores, a value ranging from 0 to 1 (Manning, Raghavan, and Schütze 2008). A purity score of 1 indicates perfect clustering alignment within clusters, while a random assignment of clusters yields purity scores close to $\frac{1}{N}$, where $N$ is the number of clusters. The results in Figures 1 to 4 present the comparison of clustering performance across datasets with varying topological weight $\lambda$. Each figure corresponds to a separate clustering task: Figure 1 displays the clustering performance when clustering connectomes from all regularization strategies and vanilla together, and Figures 2 to 4 show the clustering performances of clustering connectomes from vanilla and a regularization strategy (batch normalization, dropout, and $L^2$). For each clustering task, we performed 20 trials. The data points represent the mean purity scores across these trials, and the error bars at each point represent the standard deviations of the purity scores.

Across Figures 1 to 4, we observe an overall positive correlation between the purity scores and the topological weight $\lambda$. Generally, incorporating more topological information tends to improve clustering performance. At the left end of the figures, where $\lambda = 0$, most purity scores for Adj are close to those expected from random cluster assignments. At the right end of $\lambda = 1$, the purity scores are significantly higher across all experiments, with many approaching 1. In every clustering task, the highest purity scores occur at $\lambda = 1$, indicating optimal performance. This suggests that topological information captured by Top is effective in distinguishing the functional differences between regularization techniques.

## Experimental Setup

The experiments were conducted on a MacBook Pro with an Apple M1 Pro chip and 16 GB of unified memory. The software environment was set up using the following configurations:

- **Operating System:** macOS Sonoma 14.5
- **Processor:** Apple M1 Pro
- **Memory:** 16 GB Unified Memory
- **Programming Language:** Python 3.11.9
- **Environment Manager:** Conda 24.1.2
- **Key Libraries:**
  - NumPy 1.26.4
  - Pandas 2.2.2

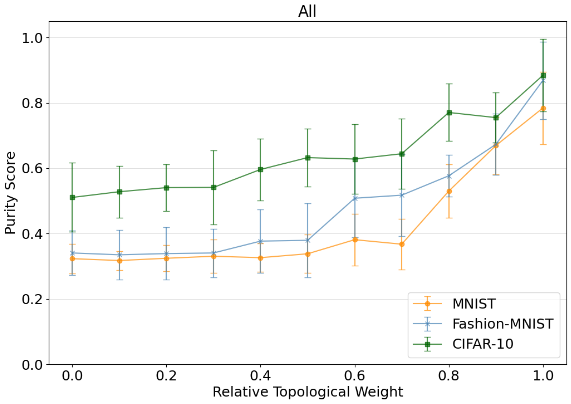


Figure 1: Purity scores of clustering connectomes of all regularization strategies into four clusters. The variation of relative topological weight $\lambda$ in the clustering method influences its performance.

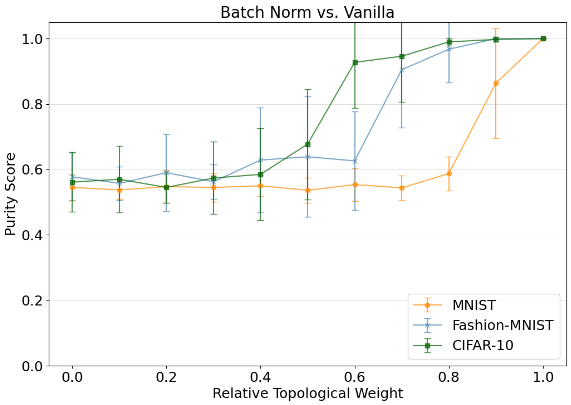


Figure 2: Purity scores of clustering connectomes of batch normalization and vanilla into two clusters with varying topological weight $\lambda$.

- SciPy 1.13.0
- Matplotlib 3.9.0
- Scikit-learn 1.5.0
- Scikit-learn-extra 0.3.0.dev0
- Torch 2.3.0
- Torchvision 0.18.0
- Ripser 0.6.8
- Persim 0.3.5

All code was executed in a conda environment to ensure reproducibility. A seed value of 42 is used for randomization in `random` (Python), `numpy`, `torch`, and functions that accept a seed input.

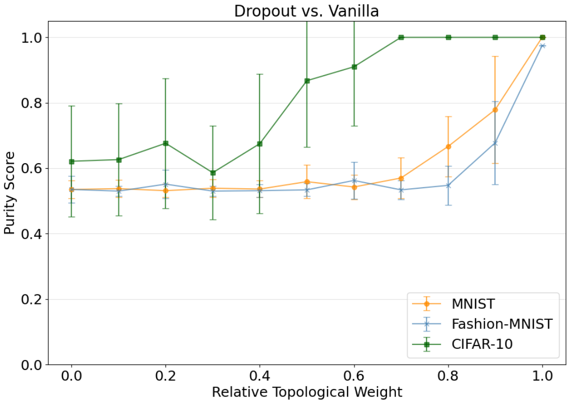


Figure 3: Purity scores of clustering connectomes of dropout and vanilla into two clusters with varying topological weight $\lambda$.

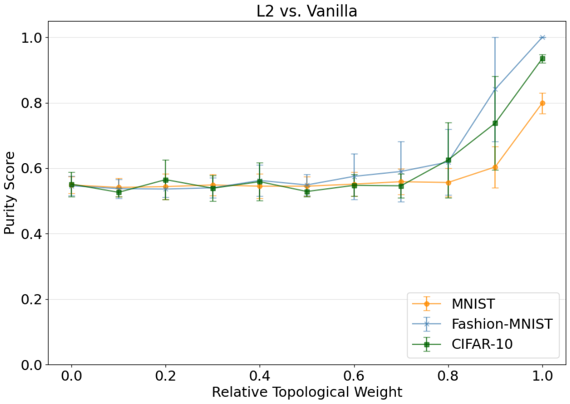


Figure 4: Purity scores of clustering connectomes of $L^2$ and vanilla into two clusters with varying topological weight $\lambda$.

## References

Adams, H.; Emerson, T.; Kirby, M.; Neville, R.; Peterson, C.; Shipman, P.; Chepushtanova, S.; Hanson, E.; Motta, F.; and Ziegelmeier, L. 2017. Persistence images: A stable vector representation of persistent homology. *Journal of Machine Learning Research*, 18(8): 1–35.

Carriere, M.; Cuturi, M.; and Oudot, S. 2017. Sliced Wasserstein kernel for persistence diagrams. In *International conference on machine learning*, 664–673. PMLR.

Hoerl, A. E.; and Kennard, R. W. 1970. Ridge regression: Biased estimation for nonorthogonal problems. *Technometrics*, 12(1): 55–67.

Ioffe, S.; and Szegedy, C. 2015. Batch normalization: Accelerating deep network training by reducing internal covariate shift. In *International conference on machine learning*, 448–456. pmlr.

Krizhevsky, A.; Hinton, G.; et al. 2009. Learning multiple layers of features from tiny images.

LeCun, Y.; Bottou, L.; Bengio, Y.; and Haffner, P. 1998. Gradient-based learning applied to document recognition. *Proceedings of the IEEE*, 86(11): 2278–2324.

Maas, A. L.; Hannun, A. Y.; Ng, A. Y.; et al. 2013. Rectifier nonlinearities improve neural network acoustic models. In *Proc. icml*, volume 30, 3. Atlanta, GA.

Manning, C. D.; Raghavan, P.; and Schütze, H. 2008. *Introduction to Information Retrieval*. Cambridge University Press.

Paszke, A.; Gross, S.; Massa, F.; Lerer, A.; Bradbury, J.; Chanan, G.; Killeen, T.; Lin, Z.; Gimelshein, N.; Antiga, L.; Desmaison, A.; Köpf, A.; Yang, E.; DeVito, Z.; Raison, M.; Tejani, A.; Chilamkurthy, S.; Steiner, B.; Fang, L.; Bai, J.; and Chintala, S. 2019. PyTorch: An Imperative Style, High-Performance Deep Learning Library. arXiv:1912.01703.

Pedregosa, F.; Varoquaux, G.; Gramfort, A.; Michel, V.; Thirion, B.; Grisel, O.; Blondel, M.; Prettenhofer, P.; Weiss, R.; Dubourg, V.; Vanderplas, J.; Passos, A.; Cournapeau, D.; Brucher, M.; Perrot, M.; and Duchesnay, E. 2011. Scikit-learn: Machine Learning in Python. *Journal of Machine Learning Research*, 12: 2825–2830.

Reininghaus, J.; Huber, S.; Bauer, U.; and Kwitt, R. 2015. A stable multi-scale kernel for topological machine learning. In *Proceedings of the IEEE conference on computer vision and pattern recognition*, 4741–4748.

Saul, N.; and Tralie, C. 2021. persim: A Python package for persistence diagrams and their similarity computations. https://github.com/scikit-tda/persim.

scikit-learn extra. 2020. scikit-learn-extra: a Python module for machine learning that extends scikit-learn.

Songdechakraiwut, T.; and Chung, M. K. 2023. Topological learning for brain networks. *The Annals of Applied Statistics*, 17(1): 403.

Songdechakraiwut, T.; Krause, B. M.; Banks, M. I.; Nourski, K. V.; and Veen, B. D. V. 2022. Fast topological clustering with Wasserstein distance. In *International Conference on Learning Representations (ICLR)*.

Srivastava, N.; Hinton, G.; Krizhevsky, A.; Sutskever, I.; and Salakhutdinov, R. 2014. Dropout: a simple way to prevent neural networks from overfitting. *The journal of machine learning research*, 15(1): 1929–1958.

TorchVision. 2016. TorchVision: PyTorch's Computer Vision library. https://github.com/pytorch/vision.

Tralie, C.; Saul, N.; and Bar-On, R. 2018. Ripser.py: A Lean Persistent Homology Library for Python. *The Journal of Open Source Software*, 3(29): 925.

Xiao, H.; Rasul, K.; and Vollgraf, R. 2017. Fashion-mnist: a novel image dataset for benchmarking machine learning algorithms. *arXiv preprint arXiv:1708.07747*.
